# Supplementary material for: Dynamics in the ordered and disordered phases of barocaloric adamantane
Source: arXiv:2210.13914 source file (2022-10-25)
Supplement: Supplementary file 1 [file SI.pdf]

# Dynamics in the ordered and disordered phases of barocaloric adamantane

Bernet E. Meijer,[a], Richard J. C. Dixey,[a] Franz Demmel,[b] Robin Perry,[c]
Helen C. Walker,[*b] and Anthony E. Phillips[*a*]

**Electronic Supplementary Information**

## Contents

**S1 Extrapolation of calorimetric data** **S2**

**S2 Inelastic neutron scattering** **S3**

**S3 Quasielastic neutron scattering under high pressure** **S5**

S3.1 Results . . . . . . . . . . . . . . . . . . . . . . . . . . . . . . . . . . . . . . . S5

S3.2 $C_4$ rotational jump model . . . . . . . . . . . . . . . . . . . . . . . . . . . . . . S6

**S4 Lattice dynamics calculations** **S8**

**S5 Brillouin zone labels** **S13**

*a.e.phillips@qmul.ac.uk, helen.c.walker@stfc.ac.uk

## S1 Extrapolation of calorimetric data

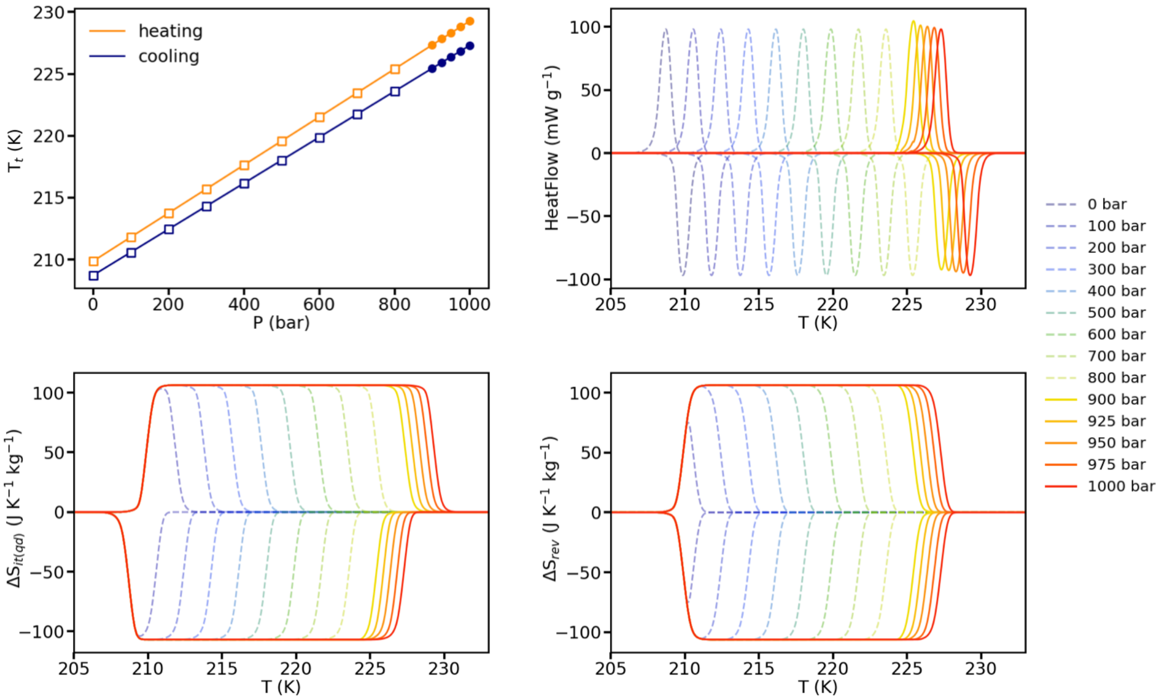


Figure S1: Details of the extrapolation of calorimetric data. (a) The phase diagram as deduced from heat-flow measurements: solid circles are experimental data points, open squares are extrapolated datapoints (based on a linear fit to the experimental data) at which the low-temperature barocaloric behaviour will be estimated. (b) Heat flow data at low pressures have been simulated by shifting the heat flow peaks from the high-pressure measurements to the predicted phase transition temperatures in (a). Solid lines are experimental data and the dotted lines are simulated. (c) The heat flow peaks are integrated and each heat flow integral for $p > 0$ is then subtracted off the heat flow integral for $p = 0$. The resulting isothermal entropy change entropy change $\Delta S_{\mathrm{it(qd)}}$ for $0 \to p$ and $p \to 0$ was scaled to correct for the increase in phase transition enthalpy at high temperatures. (d) Reversible entropy change $\Delta S_{\mathrm{rev}}$ for $0 \to p$ and $p \to 0$ deduced from (c). The simulated data predict that it is possible to get reversible barocaloric effects for pressures $< 100$ bar, with saturation already at $< 200$ bar.

## S2 Inelastic neutron scattering

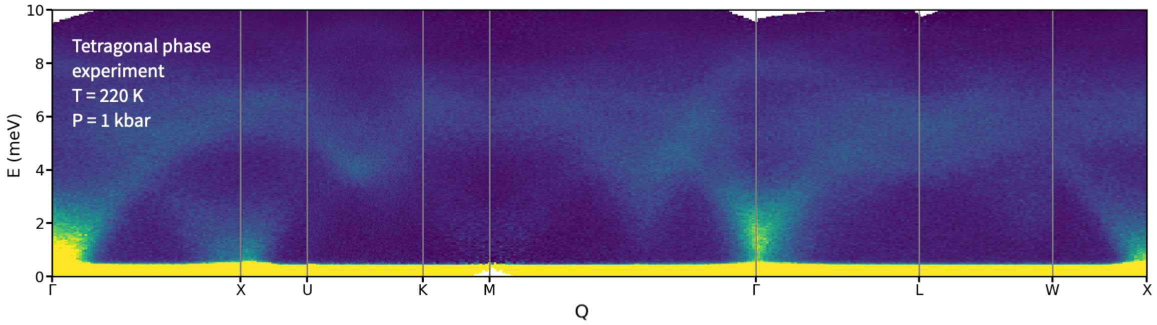


Figure S2: Dispersion curve in adamantane's ordered tetragonal phase, measured by single-crystal inelastic neutron scattering at $T = 220$ K and $P = 1$ kbar.

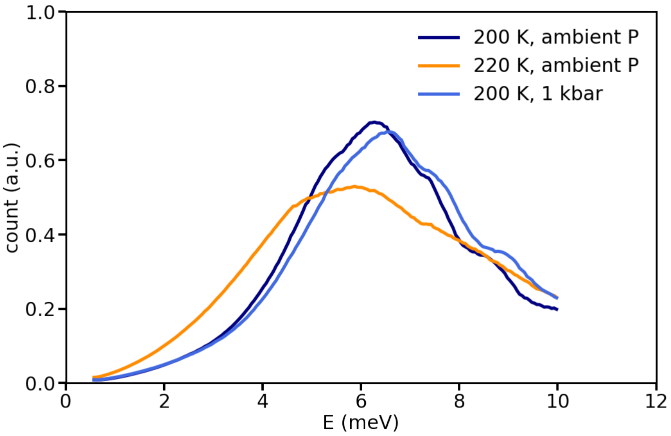


Figure S3: Experimental 1-phonon density of states. There is clear softening in the high-temperature cubic phase (220 K, ambient P) and in the tetragonal phase, the modes are stiffer at the (T=220 K, P=1 kbar) phase point than at the (T=200 K, P=ambient) phase point, likely because high pressure restricts the molecules' movements.

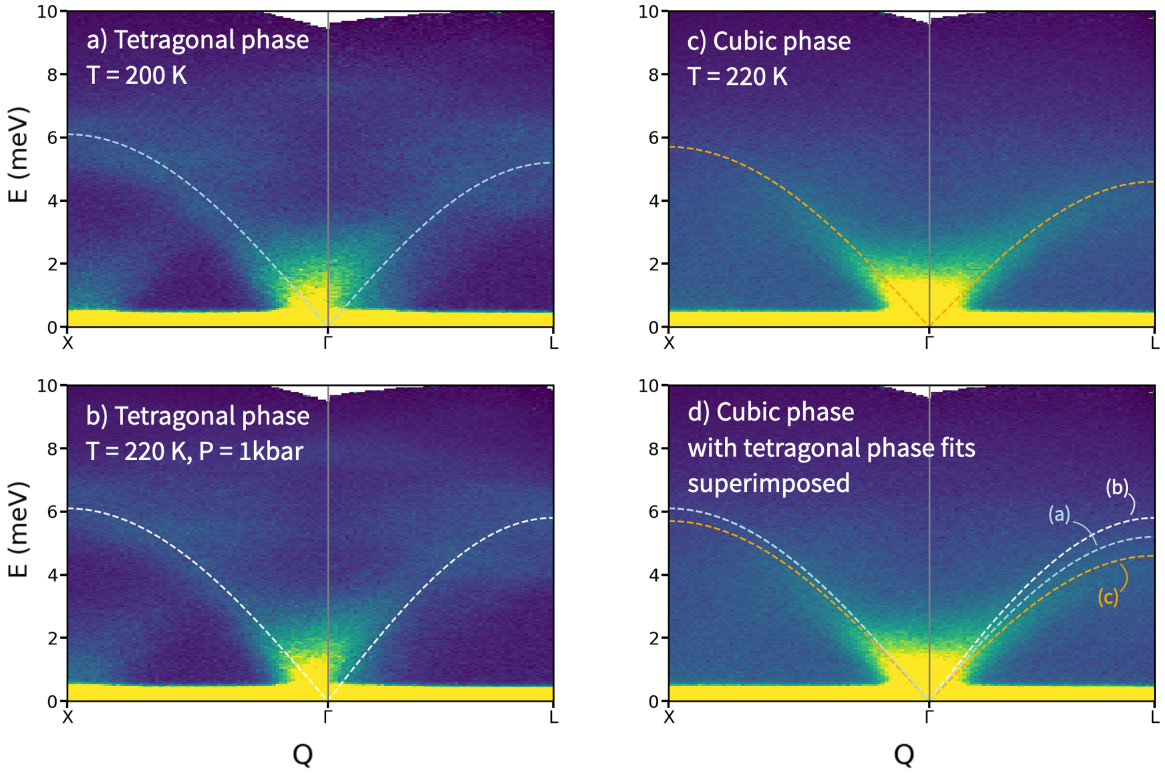


Figure S4: Acoustic modes in the experimental dispersion curves in (a) the tetragonal phase at low temperature, (b) the tetragonal phase at high pressure and (c) the cubic phase. The acoustic modes have been fitted to the eye with a sine wave of variable amplitude. The image in (d) is the cubic phase, with the fits of all phases superimposed. It shows (1) that the acoustic modes have softened in the cubic phase and (2) that the modes are stiffer in the tetragonal phase at high pressure (b) than at low temperature (a). These results are consistent with the density of states (figure S3).

## S3 Quasielastic neutron scattering under high pressure

### S3.1 Results

The model describing the quasielastic signal in adamantane's high-temperature phase has been uncovered by Bee *et al.*[1] and attributed to $C_4$ rotational jumps. In the analysis of the pressure data collected in this work, this rotational model is therefore used to fit the data. The free model parameters are $\tau_{C_4}$ (the average time between jumps), $f$ (empirical fitting parameter to account for the fraction of rotating molecules), an arbitrary scaling factor $C(Q)$ (which accounts, among others, for the Debye-Waller factor) and a background term $B(Q,\omega)$ that is assumed to be linear in the energy $\omega$. The full model is given below.

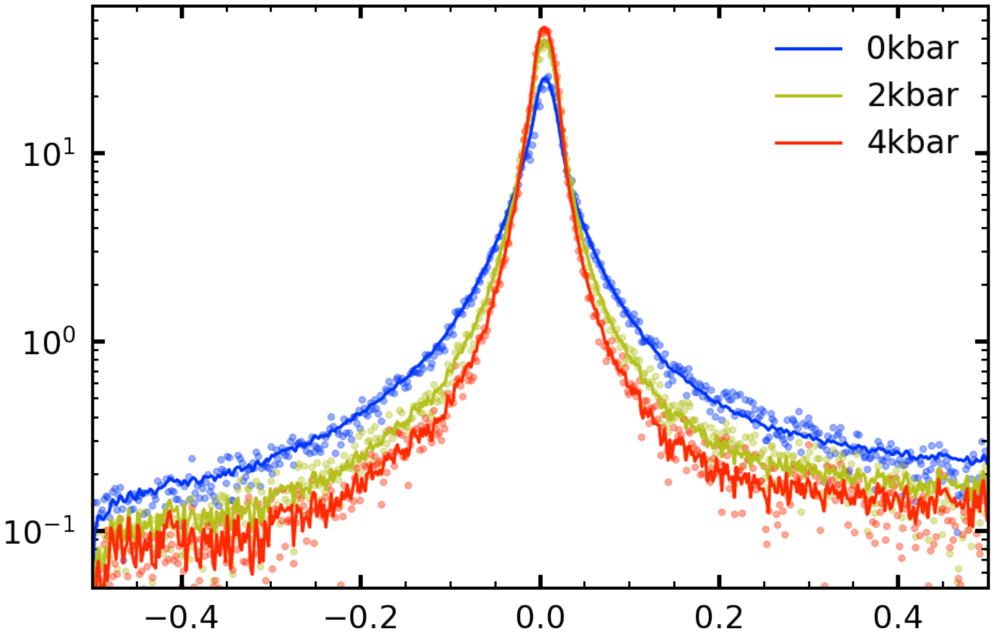


Figure S5: Quasi-elastic broadening in adamantane's disordered cubic phase is suppressed under pressure. Data were collected at $T = 300$ K. The spectra have been summed over the range 0 Å$^{-1}$< $Q$ <2 Å$^{-1}$. The experimental data are represented by dots and the corresponding fit by lines. (The fits itself contain noise due to convolution with the experimental resolution.)

The resulting fit to the pressure data is shown in figure S5. Here the spectra have been summed over all momentum transfer $Q$, to increase the signal-to-noise ratio and aid visualisation. The quasielastic broadening is suppressed by pressure. This is the result of two changing model parameters in the fit: both the frequency of $C_4$ jumps and the fraction of rotating molecules decrease with pressure, as

shown in table S3.

| $T$ (K) | $P$ (kbar) | $\tau_{C_4}$ (ps) | $f$ |
|---|---|---|---|
| 220 | 0 | 50.9 | 0.5 |
| 300 | 0 | 18.8 | 0.7 |
| 300 | 2 | 33.8 | 0.6 |
| 300 | 4 | 50.2 | 0.4 |

Table S1: Mean residence times $\tau_{C_4}$ and fraction of dynamically activated molecules as determined from a least-squares fit to the experimental spectra.

## S3.2 $C_4$ rotational jump model

The scattering function for the cubic rotational dynamics of adamantane molecules is given by an elastic contribution (represented by the delta function) plus a sum of inelastic contributions (represented by Lorentzians)[2]:

$$S(Q,\omega) = A_0(Q,f)\delta(\omega) + \sum_i A_i(Q,f)\frac{1}{\pi}\frac{1/\tau_i(\tau_{C_4})}{(1/\tau_i(\tau_{C_4}))^2+\omega^2} \tag{1}$$

The amplitudes $A_i(Q,f)$ are given by[1,2]

$$A_0(Q,f) = 1 - f + \frac{f}{24}(1+2A+B+C+2D) \tag{2}$$

$$A_1(Q,f) = \frac{f}{24}(1+2A+B-C-2D) \tag{3}$$

$$A_2(Q,f) = \frac{f}{24}(4-4A+4B) \tag{4}$$

$$A_3(Q,f) = \frac{f}{24}(9-3B+3C-6D) \tag{5}$$

$$A_4(Q,f) = \frac{f}{24}(9-3B-3C+6D) \tag{6}$$

where $f$ is the fraction of rotating molecules, and

$$A = \sum_{v=1}^{4} J_v \tag{7}$$

$$B = \sum_{v=5}^{7} J_v \tag{8}$$

$$C = \sum_{v=8}^{13} J_v \tag{9}$$

$$D = \sum_{v=14}^{16} J_v. \tag{10}$$

$J_\nu = j_0(Qr_\nu$, with $j_0(x)$ the spherical Bessel function of zeroth order and $r_\nu$ the distances between initial and final positions of atoms after various cubic rotations, calculated by Lechner and Heidemann[3]. The Lorentzian widths $\tau_i(\tau_{C_4})$ are given by

$$\frac{1}{\tau_1} = 0, \tag{11}$$

$$\frac{1}{\tau_2} = \frac{2}{\tau_{C_4}}, \tag{12}$$

$$\frac{1}{\tau_3} = \frac{1}{\tau_{C_4}}, \tag{13}$$

$$\frac{1}{\tau_4} = \frac{2}{3\tau_{C_4}}, \tag{14}$$

$$\frac{1}{\tau_5} = \frac{4}{3\tau_{C_4}}. \tag{15}$$

The theoretical scattering function has been fitted to the reduced experimental quasielastic spectra $S_{\text{exp}}(Q,\omega)$ using

$$S_{\text{exp}}(Q,\omega) = R(\omega) \otimes (C(Q)S(Q,\omega)) + B(Q,\omega), \tag{16}$$

The factor $C(Q)$ includes the Debye-Waller factor $e^{-\langle u^2 \rangle Q^2}$, where the mean-square displacement $\langle u^2 \rangle$ represents molecular vibrations and librations. $C(Q)$ was allowed to vary freely with $Q$ in the global fit. The model is convolved with the experimental resolution function $R(\omega)$ (collected with a low-temperature measurement) and a background term $B(Q,\omega)$ is added to account for inelastic contributions to the measured signal, which in this small energy range can be approximated as a linear function in energy.

## S4 Lattice dynamics calculations

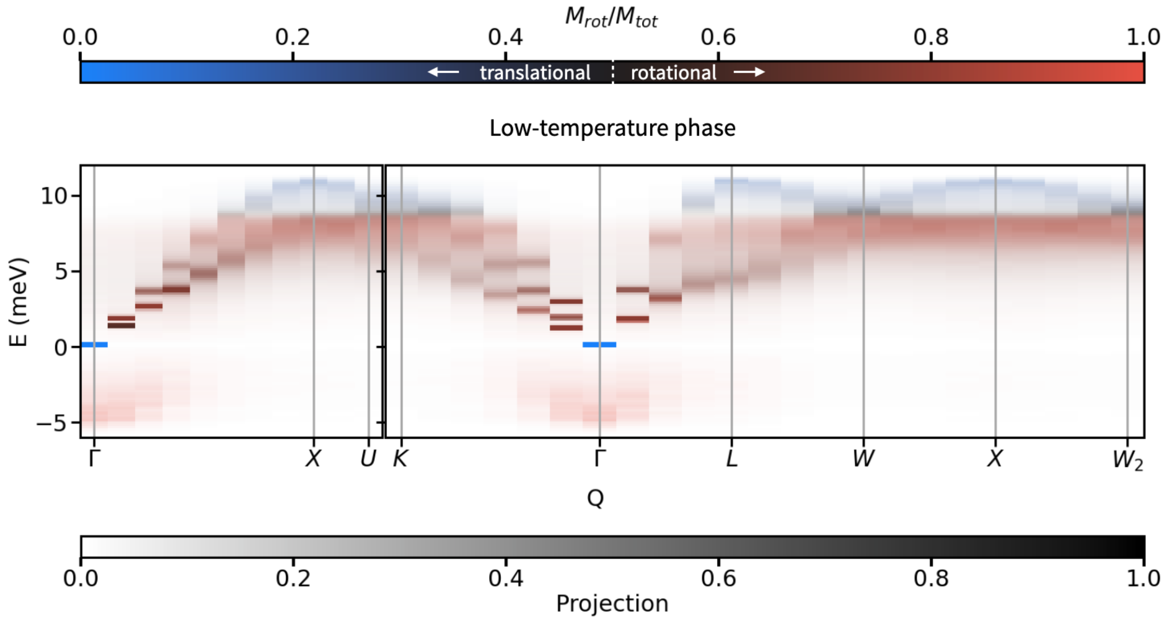


Figure S6: Dispersion curve in adamantane's disordered cubic phase calculated with supercell lattice dynamics. The imaginary frequencies have been plotted as negative frequencies. Each mode is coloured by its rotational character $M_{\mathrm{rot}}/M_{\mathrm{tot}}$. The imaginary frequencies correspond to purely rotational molecular movements.

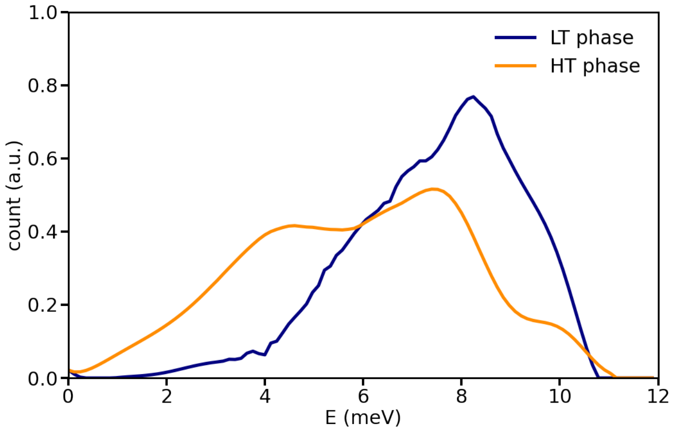


Figure S7: Calculated phonon density of states (pDOS) in adamantane's phases. In each phase, phonons were calculated at the Γ-point in a supercell ($8 \times 8 \times 8$ for high-temperature phase, $6 \times 6 \times 6$ for low-temperature phase) and projected onto the Brillouin zone; next, the projected intensities were integrated over the Brillouin zone to produce the pDOS. For the low-temperature phase, the density of states was also calculated with conventional methods (sampling the Brillouin zone with a uniform $16 \times 16 \times 16$ $k$-grid) and yielded similar results both in the shape of the pDOS and the calculated entropy (for SCLD method: $S_{\text{vib, LT}} = 695.78\ \text{JK}^{-1}\text{kg}^{-1}$; for sampling method: $S_{\text{vib, LT}} = 691.24\ \text{JK}^{-1}\text{kg}^{-1}$). The SCLD method is plotted here for consistency; this is also what is used to calculate the entropy change quoted in the main text. The imaginary frequencies (see figure S6) in the high-temperature phase have here been transformed to their absolute value; they occur around 4.5 meV.

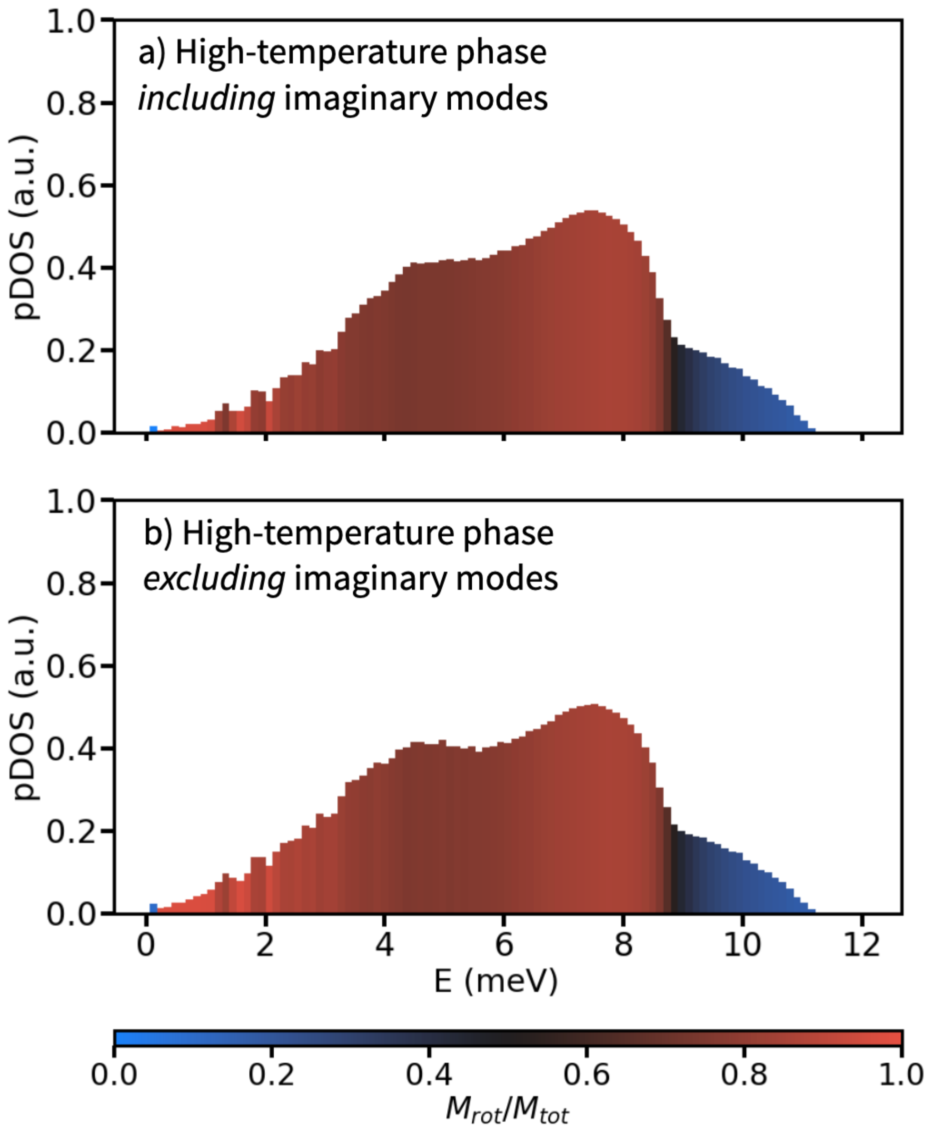


Figure S8: Difference between the calculated phonon density of states in the high temperature phase, with (a) and without (b) including imaginary modes. In (a), the imaginary frequencies have simply been transformed to their absolute values.

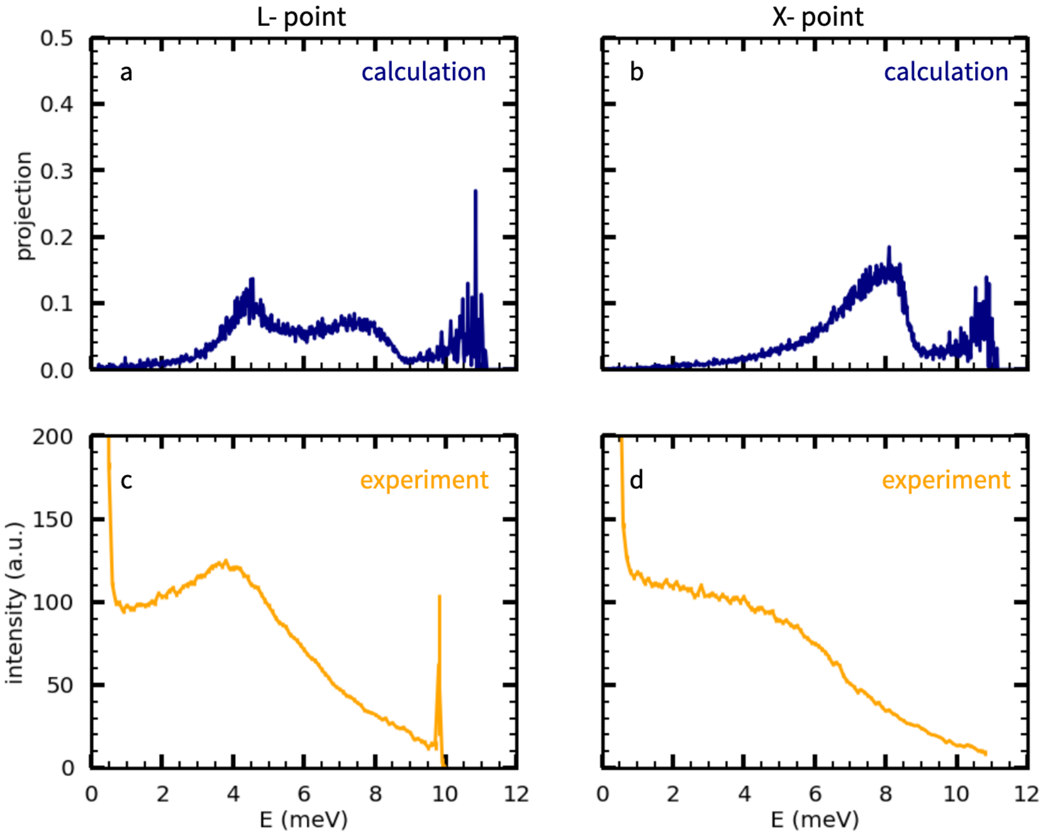


Figure S9: Comparison between cuts of the phonon spectra at chosen points in the Brillouin zone of the disordered phase. Point $L = [0.5, 0.5, 0.5]$ (integrated between $[2.25, 2.25, -3.75]$ and $[2.75, 2.75, -3.25]$ in experiment) and point $X = [0, 1.0, 0]$ (integrated between $[2.75, 2.75, -2.25]$ and $[3.25, 3.25, -1.75]$ in experiment). At the $L$-point, the feature at 4 meV is reproduced. Features at higher energies do not occur in the experiment, likely because of neutron weighting. Neutron weighting has not been accounted for in the calculation of the disordered phase since neutron weighting software is currently not compatible with the SCLD method. However, the neutron weighting in the ordered phase (figure S10) shows that high-energy modes are downweighted in the neutron structure factor. This will likely be replicated in the disordered phase, which explains the absence of high-energy features in the experimental neutron data.

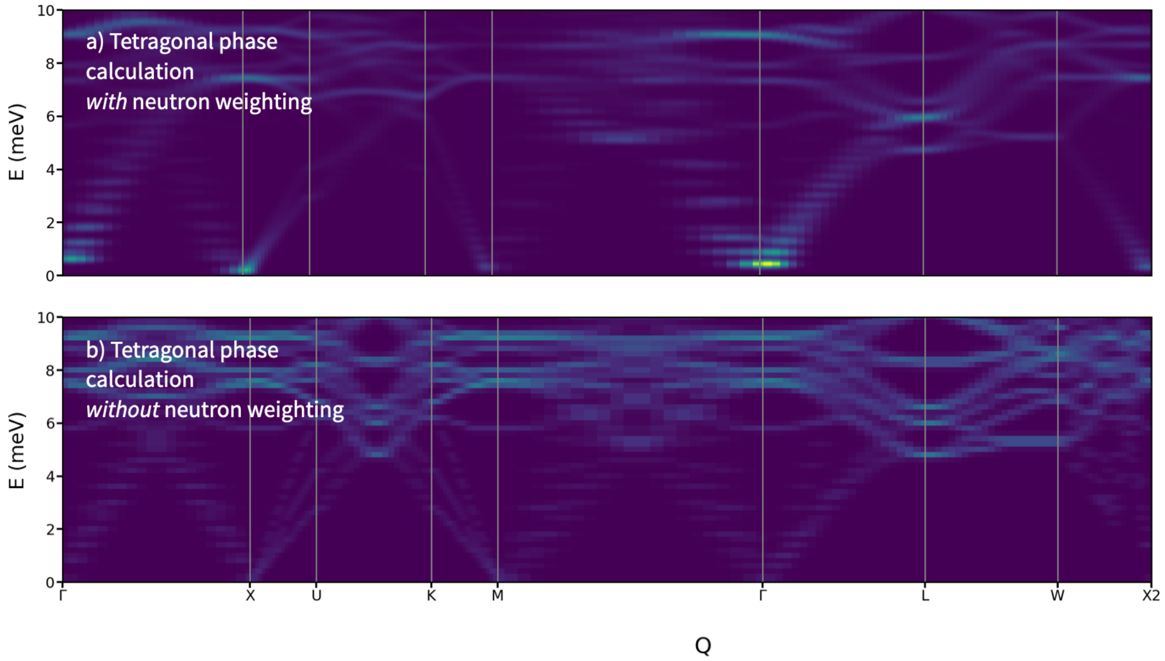


Figure S10: Calculated dispersion relation of adamantane's low-temperature phase, with (a) and without (b) neutron weighting. Most of the high-energy (> 5 meV) features are down-weighted in the neutron structure factor.

## S5 Brillouin zone labels

| Point | Wavevector coordinates |
|---|---|
| Γ | $[0, 0, 0]$ |
| X | $[0, 1, 0]$ |
| L | $[0.5, 0.5, 0]$ |
| W | $[0.5, 1, 0]$ |
| U | $[0.25, 1, 0.25]$ |
| $W_2$ | $[0, 1, 0.5]$ |
| K | $[0.75, 0, 0.75]$ |

Table S2: Labels of high-symmetry points in the Brillouin zone of space group $Fm\bar{3}m$. Wavevector coordinates are in conventional basis. In the neutron experiment, the path using these points was centred at $\Gamma = [3, 3, -3]$.

| Point | Wavevector coordinates |
|---|---|
| Γ | $[0, 0, 0]$ |
| X | $[0, 0.5, 0]$ |
| M | $[0.5, 0.5, 0]$ |
| Z | $[0, 0, 0.5]$ |
| R | $[0, 0.5, 0.5]$ |
| A | $[0.5, 0.5, 0.5]$ |

Table S3: Labels of high-symmetry points in the Brillouin zone of space group $P\bar{4}2_1c$.

## References


[1] M. Bee, J. P. Amoureux, R. E. Lechner, *Molecular Physics* **1980**, *40*, 617–641.

[2] M. M. Bée, *Quasielastic neutron scattering : principles and applications in solid state chemistry, biology, and materials science*, Adam Hilger, **1988**, p. 437.

[3] R. E. Lechner, A. Heidemann, *Commun. Phys.* **1976**, *1*, 213.
